# Supplementary material for: Dissipative Hamiltonian Neural Networks: Learning Dissipative and Conservative Dynamics Separately
Source: arXiv:2201.10085 source file (2022-01-26)
Supplement: Supplementary file 1 [file appendix.tex]

\section{Supplementary Figures}

\begin{figure*}[ht!]
\centering
\includegraphics[width=\textwidth]{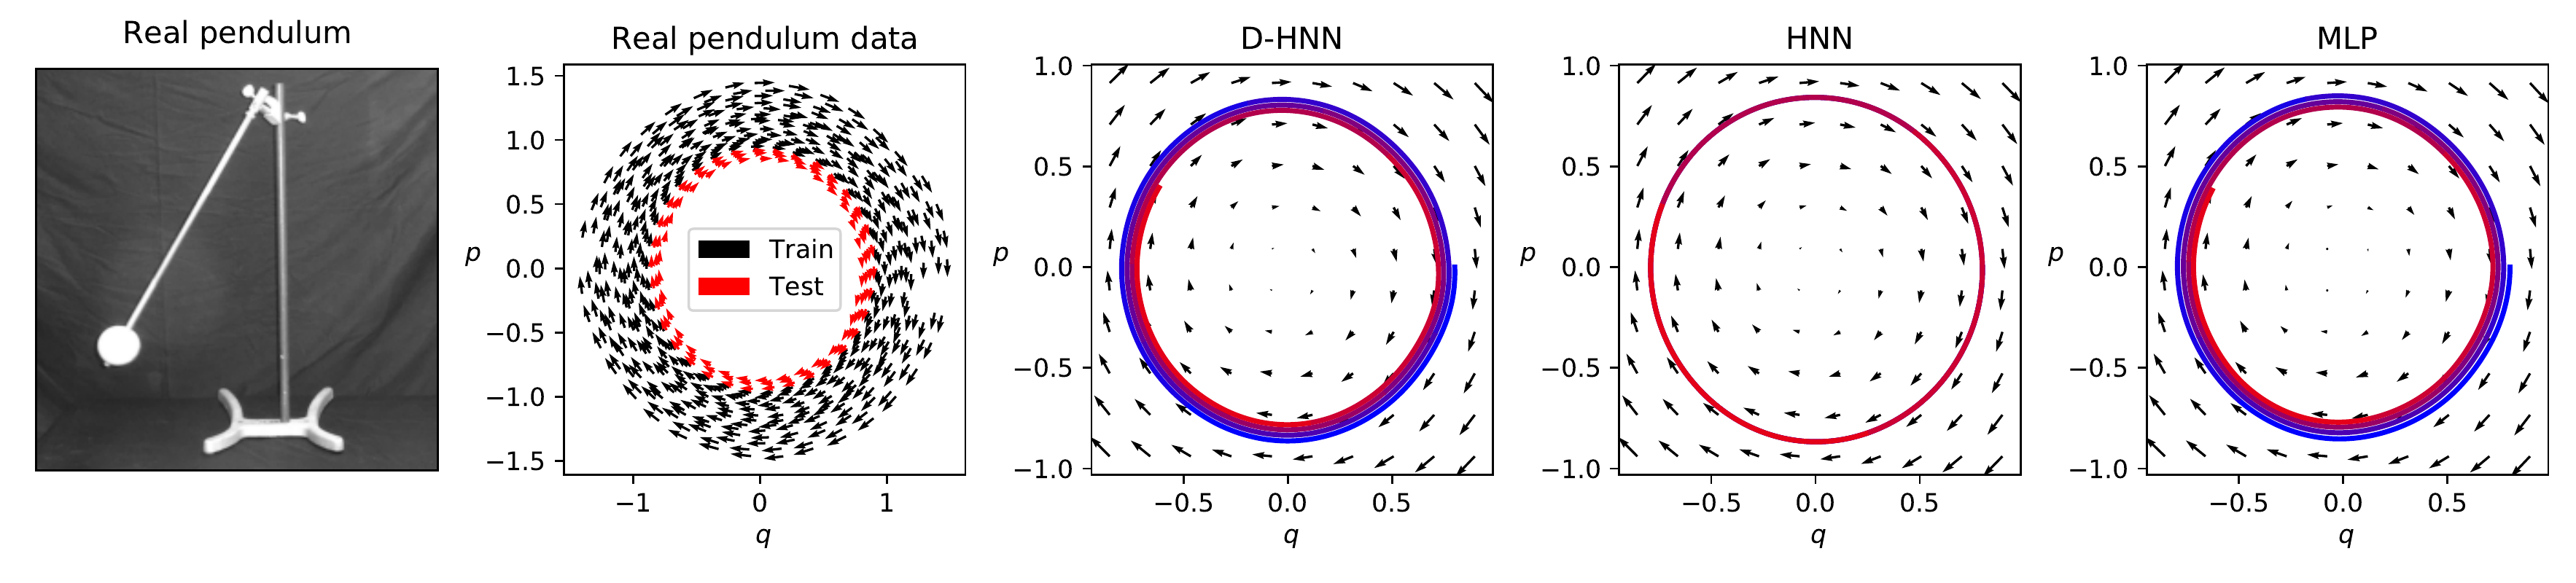}
\caption{Visualizing the experimental setup and predicted dynamics for the real pendulum experiment.}
\label{fig:realpend}
\end{figure*}

\begin{figure*}[ht!]
\centering
\includegraphics[width=\textwidth]{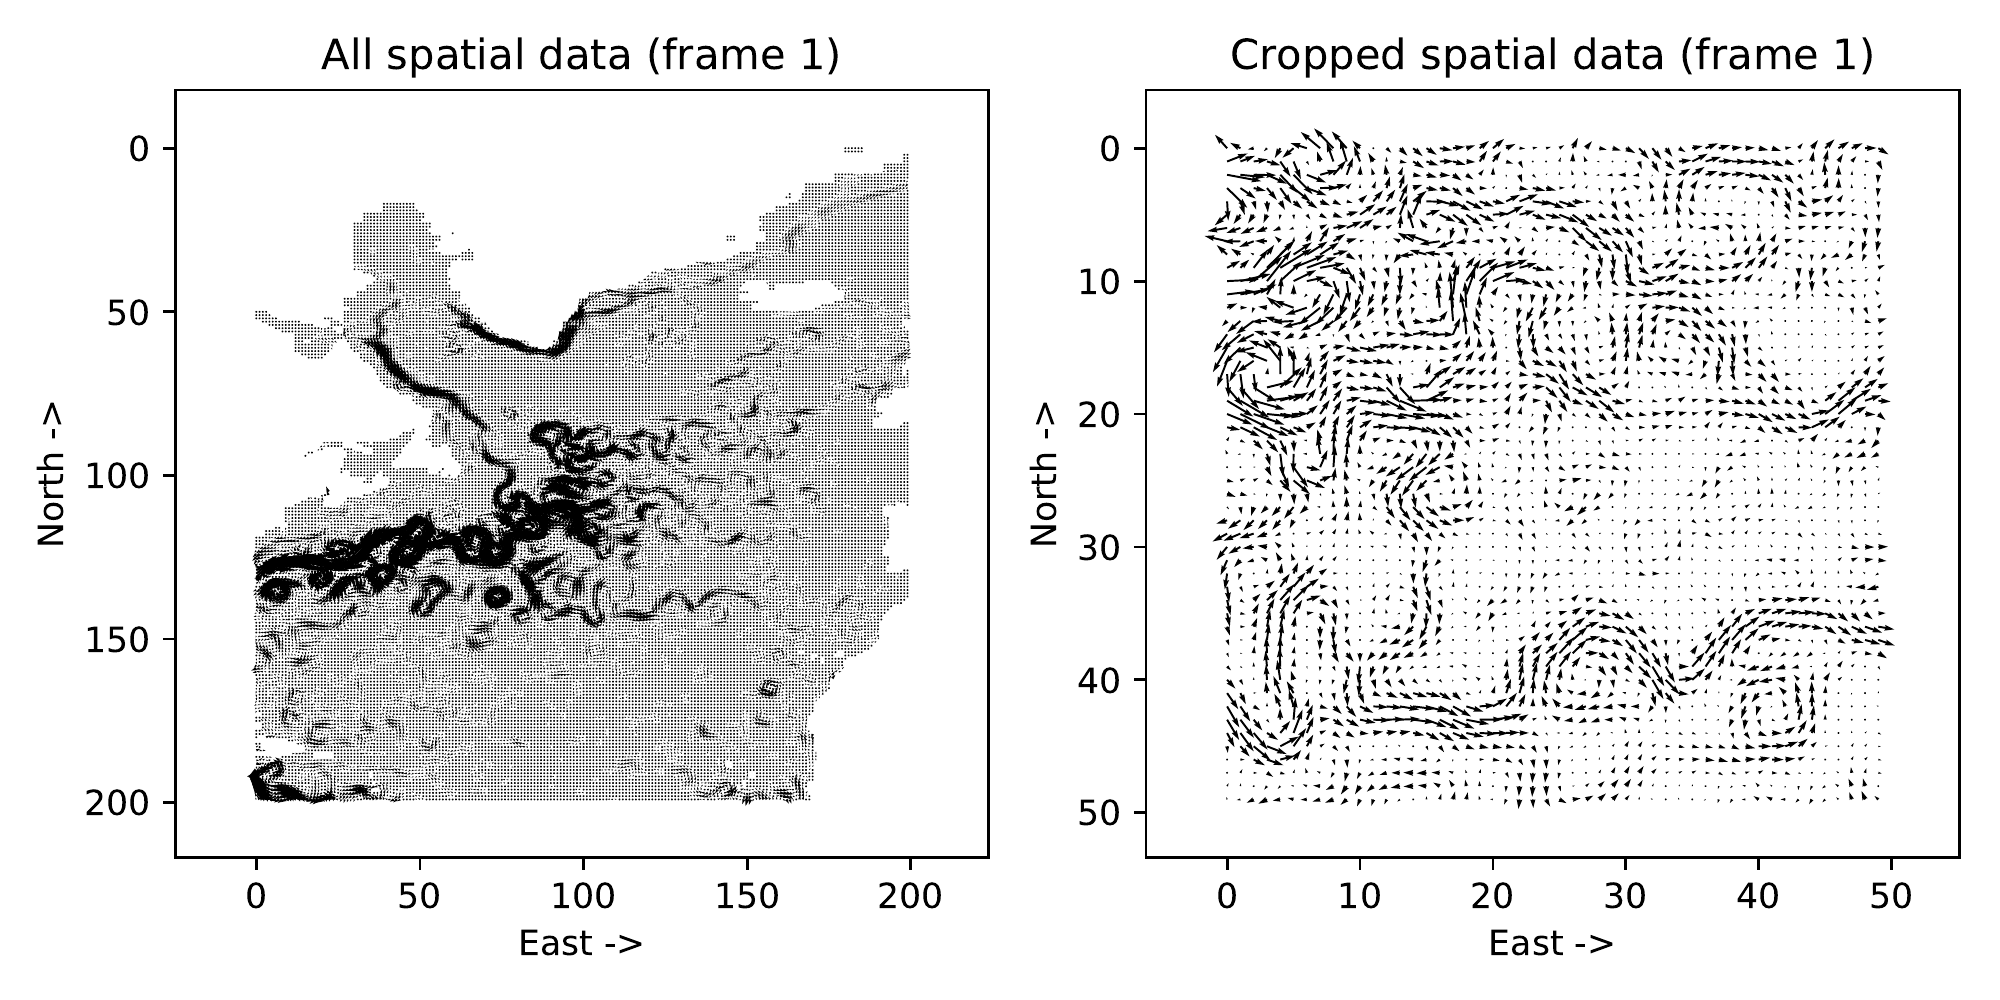}
\caption{First frame of ocean data. Oceanographers are typically interested in modeling ocean flow velocity fields and identifying features such eddy currents, upwelling and downwelling. \textbf{Left:} Surface current velocities in the Atlantic Ocean. \textbf{Right:} For our experiment, we cropped a 50x50 grid of surface currents from the middle of the Atlantic Ocean to use as training data for our models.}
\label{fig:ocean_data}
\end{figure*}

\section{Ocean Dataset} \label{sec:Ocean Dataset}

For Task 3, we tested the performance of D-HNNs on the Ocean Surface Current Analysis Real-time (OSCAR) dataset \cite{ESR2009} because we wanted to showcase how D-HNNs can decompose large, complex dynamical systems and unlock broader scientific insights about the data. The OSCAR mission is conducted by Earth Space Research and funded by NASA. The full dataset included five main variables:
\begin{itemize}
  \item Latitudinal and longitudinal coordinates $(\textbf{x}, \textbf{y})$
  \item Zonal and meridional current velocities $(\textbf{u}, \textbf{v})$
  \item Time $\textbf{t}$
\end{itemize}
According to \citet{ESR2009} these data were collected from the various satellites and in situ instruments. Data are on a 1/3 degree grid with a 5 day resolution, recorded from January 1, 2020 to December 10\textsuperscript{th}, 2020, which results in 69 time frames. The entire dataset contained  69 x 481 x 1201 points, which should be interpreted as 69 time frames of surface current velocities that span the entire range of longitudes and latitudes. For our experiment, we cropped a 50x50 grid (rows 100-150, columns 50-100) of surface currents from the middle of the Atlantic Ocean (see Figure \ref{fig:ocean_data}), and thus the size of the dataset for our experiment was 69x50x50.  More information about the OSCAR dataset can be found at \url{ https://www.esr.org/research/oscar/oscar-surface-currents/}. One can make an Earth Resource account and download the dataset from the Physical Oceanography Distributed Active Archive Center at \url{podaac-tools.jpl.nasa.gov/drive/files/allData/oscar/preview/L4/oscar_third_deg}.

\section{Hyperparameters} \label{sec:hypers}

On the damped spring task we lowered the learning rate of the HNN model from 1e-2 to 5e-3 because the slightly higher learning rate of 1e-2 was causing the vector field to become extremely rough. This is due to the fact that the data had a non-trivial dissipative component that the HNN was unable to model using its symplectic gradient field.

\begin{table}[h!]
\caption{Default hyperparameters.}
\label{tab:inner-hypers}
\begin{center} \begin{small} \begin{sc}
\begin{tabular}{ll}
\toprule
Hyperparameter & Value \\
\midrule
Train/test split    &  80\%  \\
Hidden neurons    &  256  \\
Learning rate    &  $1 \times 10^{-2}$  \\
Batch size    &  128  \\
Training steps   &  5000  \\
Input dimension    &  3  \\
Output dimension    &  2  \\
Weight decay & 0 \\ %$1 \times 10^{-5}$ \\ 
Seed    &  42  \\
\bottomrule
\end{tabular}
\end{sc} \end{small} \end{center}

\end{table}
